# Supplementary material for: Avoiding The Man on the Wire: Improving Tor's Security with Trust-Aware Path Selection
Source: arXiv:1511.05453 source file (2017-01-27)
Supplement: Supplementary file 1 [file appendix.tex]

\appendix
\appendixpage

\section{Comments}
